# Supplementary material for: When Adaptation Hurts: Connecting Representational Drift to OOD Failures in MedSAM Fine-Tuning
Source: arXiv:2608.21300 source file (2026-08-29)
Supplement: Supplementary file 1 [file SAFER_003_supp.tex]

% MICCAI 2026 / LNCS version merged from current draft.
% For initial MICCAI submission, keep authors anonymized.
% For camera-ready, replace the anonymized author block with the real author block below.

\documentclass[runningheads]{llncs}

\usepackage[T1]{fontenc}
\usepackage{graphicx}
\usepackage{booktabs}
\usepackage{multirow}
\usepackage{makecell}
\usepackage{longtable}
\usepackage{placeins}
\usepackage{rotating}
\usepackage{appendix}
\usepackage{graphicx}
\usepackage{subcaption}
\usepackage{comment}
\usepackage{float}
\usepackage{placeins}
\usepackage{dblfloatfix}
\usepackage{array}
\usepackage{url}

\makeatletter
\newcommand{\printfnsymbol}[1]{%
  \textsuperscript{\@fnsymbol{#1}}%
}
\makeatother

\begin{document}

\newcommand{\maketitlesupplementary}{
\begin{center}
{\Large \bfseries When Adaptation Hurts: Connecting Representational Drift to OOD Failures in MedSAM Fine-Tuning.\par}
\vspace{1.0em}
{\Large \bfseries Supplementary Material\par}
\end{center}
\vspace{1.5em}
}

\clearpage
\appendix
\maketitlesupplementary
\FloatBarrier



\input{Sections/appendix/A_0_bbox_increase_by_jitter}
\input{Sections/appendix/A_1_additional_hd95_results}
\input{Sections/appendix/B_cka_analysis}
% \input{Sections/appendix/C_cka_aware_ft_loss}
% \input{Sections/appendix/D_seg_performance_perfect_bboxes}
%\input{Sections/appendix/E_dice_cka_across_jitters_big_table}
\input{Sections/appendix/F_segmentation_perf_bbox_expansion}
\input{Sections/appendix/G_dice_across_jitters_big_table}


\end{document}
