# Supplementary material for: When Adaptation Hurts: Connecting Representational Drift to OOD Failures in MedSAM Fine-Tuning
Source: arXiv:2608.21300 source file (2026-08-29)
Supplement: Supplementary file 5 [file C_cka_aware_ft_loss.tex]

\section{CKA aware fine tuning auxiliary loss}
\label{subsec:cka_aware_finetuning}

We introduce a CKA based auxiliary loss to regularize fine tuning toward the internal representations of the frozen base MedSAM model. This regularizer does not force the fine tuned model to reproduce base MedSAM outputs, but instead discourages excessive internal representation drift while allowing the segmentation loss to adapt the model to the target domain. The standard segmentation objective is the Dice and BCE loss used throughout training:
\begin{equation}
\mathcal{L}_{\mathrm{task}} =
(1 - w_{\mathrm{dice}})\mathcal{L}_{\mathrm{BCE}}
+ w_{\mathrm{dice}}\mathcal{L}_{\mathrm{Dice}},
\end{equation}
with \(w_{\mathrm{dice}} = 0.5\) in our experiments.

For a hooked layer \(l\), let \(X_l\) denote the activation matrix from frozen MedSAM and \(Y_l\) the corresponding activation matrix from the fine tuned model on the same fixed probe batch. After flattening activations, linear CKA is computed as
\begin{equation}
\mathrm{CKA}(X_l,Y_l) =
\frac{\left\|X_l^\top Y_l\right\|_F^2}
{\left\|X_l^\top X_l\right\|_F
\left\|Y_l^\top Y_l\right\|_F}.
\end{equation}
The layer penalty is therefore
\begin{equation}
\mathcal{L}_{\mathrm{CKA},l} =
1 - \mathrm{CKA}(X_l,Y_l),
\end{equation}
which penalizes representational drift from the base model.

For multiple hooked layers \(H\), we use a weighted CKA loss:
\begin{equation}
\mathcal{L}_{\mathrm{CKA}} =
\sum_{l \in H} \alpha_l
\left(1 - \mathrm{CKA}(X_l,Y_l)\right),
\end{equation}
where \(\alpha_l\) controls the contribution of each layer. The final objective is
\begin{equation}
\mathcal{L}_{\mathrm{total}} =
\mathcal{L}_{\mathrm{task}} +
\lambda \mathcal{L}_{\mathrm{CKA}}.
\end{equation}

The CKA loss is computed on a fixed multi domain probe set, while base MedSAM activations are cached once before training. During optimization, the task loss and CKA loss are backpropagated separately before a single optimizer step, which is equivalent to optimizing \(\mathcal{L}_{\mathrm{total}}\) but reduces memory use. To further reduce cost, the CKA term is applied every \(N\) steps with an effective weight \(\lambda_{\mathrm{eff}} = N\lambda\). 
