# Supplementary material for: When Adaptation Hurts: Connecting Representational Drift to OOD Failures in MedSAM Fine-Tuning
Source: arXiv:2608.21300 source file (2026-08-29)
Supplement: Supplementary file 6 [file D_seg_performance_perfect_bboxes.tex]

\section{Segmentation performance of models trained and evaluated on perfect bounding boxes}
\label{sec:seg_perf_clean}

Table~\ref{tab:combined_finetuning_all_datasets} compares all methods trained and evaluated with exact ground-truth bounding boxes ($p_m{=}0$), reporting Dice, HD95, and IoU across all four datasets. Using perfect prompts removes noise from the comparison, so differences in performance reflect the adaptation strategy rather than prompt quality.

On ISIC 2018 and close-OOD PH$^2$, all methods improve over zero-shot MedSAM and the rankings are fairly stable. LoRA+CKA achieves the best in-domain Dice. It achieves scores of $0.966$, HD95 $0.302$ px, while encoder-only LoRA takes the top spot on PH$^2$ with a value of $0.961$. VPT variants and decoder-only are a few points behind. They cluster between Dice $0.943$ and $0.949$ across both datasets.

The far-OOD results tell a different story. On BUSI the VPT-shallow, VPT-deep, standard LoRA, and LoRA+CKA methods all drop below zero-shot, which has a value of $0.823$. For far-OOD, HD95 values can reach up to $172.290$ px in the worst case for LoRA compared to $20.420$ px for zero-shot. Encoder-only LoRA and full fine-tuning outperform zero-shot on both far-OOD datasets. Decoder-only also performs well on far-OOD, nearly matching full fine-tuning on CBIS-DDSM while only updating the decoder weights. Decoder-only scores $0.828$, which is close to the CBIS-DDSM's performance of $0.829$. It must be noted that this was exhibited only in the perfect bounding box scenario, while at any perturbation level applied to the input prompt, decoder-only training produced much worse predictions and remained unstable. More detailed analysis follows in Section~\ref{sec:degration_w_jitter}


\begin{table}[H]
\centering
\scriptsize
\setlength{\tabcolsep}{3pt}
\renewcommand{\arraystretch}{1.05}
\begin{tabular}{llcccc}
\toprule
\textbf{Dataset} & \textbf{Method} & \textbf{Dice $\uparrow$} & \textbf{HD95 $\downarrow$} & \textbf{IoU $\uparrow$} & \textbf{Params $\downarrow$} \\
\midrule
\multirow{8}{*}{\makecell{ISIC 2018 \\ \textit{trained on}}}
& Zero-shot    & $0.907 \pm 0.064$ & $14.610$ px & $0.836$ & $0.000$ M \\
& Decoder-only & $0.949 \pm 0.043$ & $5.330$ px  & $0.905$ & $4.058$ M \\
& VPT-shallow  & $0.945 \pm 0.044$ & $5.930$ px  & $0.899$ & $4.066$ M \\
& VPT-deep     & $0.947 \pm 0.043$ & $5.560$ px  & $0.902$ & $4.151$ M \\
& LoRA         & $0.956 \pm 0.041$ & $3.890$ px & $0.918$ & $4.353$ M \\
& LoRA + CKA late  & $\mathbf{0.966 \pm 0.017}$ & $\mathbf{0.302}$ px & $\mathbf{0.936}$ & $4.353$ M \\
& LoRA Encoder-only & $0.957 \pm 0.031$ & $\underline{1.517}$ px & $0.920$ & $4.129$ M \\
& Full FT & $\underline{0.961 \pm 0.036}$ & $2.580$ px & $\underline{0.927}$ & $93.730$ M \\
\midrule
\multirow{8}{*}{\makecell{PH$^2$ \\ \textit{close OOD}}}
& Zero-shot    & $0.905 \pm 0.076$ & $17.000$ px & $0.834$ & $0.000$ M \\
& Decoder-only & $0.947 \pm 0.033$ & $5.100$ px  & $0.901$ & $4.058$ M \\
& VPT-shallow  & $0.943 \pm 0.034$ & $5.200$ px  & $0.895$ & $4.066$ M \\
& VPT-deep     & $0.946 \pm 0.032$ & $4.900$ px  & $0.898$ & $4.151$ M \\
& LoRA         & $0.957 \pm 0.026$ & $\underline{2.500}$ px & $0.919$ & $4.353$ M \\
& LoRA + CKA late & $\underline{0.959 \pm 0.024}$ & $\mathbf{1.889}$ px & $\underline{0.923}$ & $4.353$ M \\
& LoRA Encoder-only & $\mathbf{0.961 \pm 0.024}$ & $\underline{2.060}$ px & $\mathbf{0.925}$ & $4.129$ M \\
& Full FT & $0.958 \pm 0.026$ & $2.600$ px & $0.921$ & $93.730$ M \\
\midrule
\multirow{8}{*}{\makecell{BUSI \\ \textit{far OOD}}}
& Zero-shot    & $0.823 \pm 0.088$ & $20.420$ px  & $0.708$ & $0.000$ M \\
& Decoder-only & $0.894 \pm 0.067$ & $14.900$ px  & $0.813$ & $4.058$ M \\
& VPT-shallow  & $0.792 \pm 0.154$ & $169.100$ px & $0.679$ & $4.066$ M \\
& VPT-deep     & $0.802 \pm 0.154$ & $142.860$ px & $0.692$ & $4.151$ M \\
& LoRA         & $0.780 \pm 0.190$ & $172.290$ px & $0.673$ & $4.353$ M \\
& LoRA + CKA late  & $0.813 \pm 0.145$ & $117.151$ px & $0.705$ & $4.353$ M \\
& LoRA Encoder-only & $\mathbf{0.906 \pm 0.062}$ & $\mathbf{11.038}$ px & $\mathbf{0.833}$ & $4.129$ M \\
& Full FT & $\underline{0.901 \pm 0.065}$ & $\underline{12.000}$ px & $\underline{0.825}$ & $93.730$ M \\
\midrule
\multirow{8}{*}{\makecell{CBIS-DDSM \\ \textit{far OOD}}}
& Zero-shot    & $0.692 \pm 0.164$ & $15.300$ px  & $0.551$ & $0.000$ M \\
& Decoder-only & $\underline{0.828 \pm 0.129}$ & $9.800$ px & $\mathbf{0.721}$ & $4.058$ M \\
& VPT-shallow  & $0.566 \pm 0.249$ & $184.300$ px & $0.436$ & $4.066$ M \\
& VPT-deep     & $0.573 \pm 0.243$ & $173.600$ px & $0.438$ & $4.151$ M \\
& LoRA         & $0.509 \pm 0.276$ & $243.600$ px & $0.387$ & $4.353$ M \\
& LoRA + CKA late  & $0.536 \pm 0.242$ & $252.702$ px & $0.402$ & $4.353$ M \\
& LoRA Encoder-only & $0.805 \pm 0.124$ & $\underline{9.512}$ px & $0.687$ & $4.129$ M \\
& Full FT & $\mathbf{0.829 \pm 0.124}$ & $\mathbf{8.200}$ px & $\mathbf{0.721}$ & $93.730$ M \\
\bottomrule
\end{tabular}
\caption{Comparison of fine-tuning methods across ISIC 2018, PH$^2$, BUSI, and CBIS-DDSM datasets. Baseline rows are averaged over 3 random seeds. The $\pm$ values denote per-image Dice standard deviation across the evaluation set. Training used the exact tight ground-truth bounding box ($p_m{=}0$).}
\label{tab:combined_finetuning_all_datasets}
\end{table}
