# Supplementary material for: When Adaptation Hurts: Connecting Representational Drift to OOD Failures in MedSAM Fine-Tuning
Source: arXiv:2608.21300 source file (2026-08-29)
Supplement: Supplementary file 7 [file E_dice_cka_across_jitters_big_table.tex]

\section{Dice and CKA per method across training and evaluation jitters}

Table~\ref{tab:perf_cka_jitter_train0} shows that the CKA-aware variant of LORA improves performance under clean bounding box dimensions. However, the drop in dice-scores is steeper than other LoRA methods once the jitter of the bounding box becomes larger. This is most prevalent for the far-OOD datasets. For this reason the LoRA method using CKA aware loss is excluded from further analysis. 

{
\small
\begin{longtable}[H]{lllcccccc}
\caption{Performance and CKA under bounding-box jitter for models trained with zero jitter only. Dice performance and CKA are reported at zero jitter, averaged across evaluation jitters, and at 200 px jitter.}
\label{tab:perf_cka_jitter_train0}\\
\toprule
Dataset & Training & Method & Dice@0 & mDice & Dice@200 & CKA@0 & mCKA & CKA@200 \\
\midrule

\multirow{8}{*}{\makecell{ISIC 2018 \\ \textit{ID}}} 
& 0 & Zero-shot & 0.9072 & \underline{0.9019} & 0.7673 & 1.0000 & 1.0000 & 1.0000 \\
&   & Decoder-only & 0.9487 & 0.8798 & 0.7075 & \textbf{0.9462} & \textbf{0.9432} & \textbf{0.9330} \\
&   & VPT-shallow & 0.9457 & 0.8858 & 0.7306 & \underline{0.8845} & \underline{0.8908} & \underline{0.8913} \\
&   & VPT-deep & 0.9472 & 0.8863 & 0.7256 & 0.8767 & 0.8791 & 0.8718 \\
&   & LoRA & 0.9545 & 0.9015 & \underline{0.7978} & 0.5685 & 0.5794 & 0.5771 \\
&   & LoRA CKA aware & \textbf{\underline{0.9664}} & 0.8508 & 0.6303 & 0.7843 & 0.7798 & 0.7713 \\
&   & LoRA Encoder-only & 0.9580 & 0.8435 & 0.6450 & 0.6484 & 0.6462 & 0.6379 \\
&   & Full FT & 0.9609 & 0.8924 & 0.7098 & 0.7755 & 0.7738 & 0.7609 \\

\midrule

\multirow{8}{*}{\makecell{PH$^2$ \\ \textit{near-OOD}}} 
& 0 & Zero-shot & 0.9054 & 0.9004 & 0.7986 & 1.0000 & 1.0000 & 1.0000 \\
&   & Decoder-only & 0.9466 & 0.8802 & 0.7269 & \textbf{0.9423} & \textbf{0.9385} & \textbf{0.9314} \\
&   & VPT-shallow & 0.9436 & 0.8846 & 0.7485 & \underline{0.8905} & \underline{0.8958} & \underline{0.8933} \\
&   & VPT-deep & 0.9458 & 0.8883 & 0.7463 & 0.8825 & 0.8810 & 0.8765 \\
&   & LoRA & 0.9557 & \underline{0.9053} & \underline{0.8342} & 0.5716 & 0.5766 & 0.5733 \\
&   & LoRA CKA aware & 0.9594 & 0.8906 & 0.7379 & 0.7853 & 0.7789 & 0.7712 \\
&   & LoRA Encoder-only & \textbf{\underline{0.9598}} & 0.8804 & 0.7528 & 0.6535 & 0.6466 & 0.6331 \\
&   & Full FT & 0.9583 & 0.8898 & 0.7437 & 0.8258 & 0.8201 & 0.8064 \\

\midrule

\multirow{8}{*}{\makecell{CBIS-DDSM \\ \textit{far-OOD}}} 
& 0 & Zero-shot & 0.6924 & \textbf{\underline{0.5986}} & \textbf{\underline{0.1889}} & 1.0000 & 1.0000 & 1.0000 \\
&   & Decoder-only & 0.8273 & 0.5076 & 0.1570 & \underline{0.9353} & \underline{0.9339} & \underline{0.9345} \\
&   & VPT-shallow & 0.6388 & 0.4264 & 0.1461 & 0.8278 & 0.8361 & 0.8531 \\
&   & VPT-deep & 0.5744 & 0.3876 & 0.1336 & 0.7996 & 0.8104 & 0.8221 \\
&   & LoRA & 0.4979 & 0.3795 & 0.1433 & 0.7624 & 0.7710 & 0.7882 \\
&   & LoRA CKA aware & 0.5360 & 0.2876 & 0.0339 & 0.7816 & 0.7856 & 0.7959 \\
&   & LoRA Encoder-only & 0.7926 & 0.5358 & 0.1872 & 0.9073 & 0.9070 & 0.9092 \\
&   & Full FT & \textbf{\underline{0.8280}} & 0.5480 & 0.1704 & \textbf{0.9479} & \textbf{0.9487} & \textbf{0.9533} \\

\midrule

\multirow{8}{*}{\makecell{BUSI \\ \textit{far-OOD}}} 
& 0 & Zero-shot & 0.8234 & \textbf{\underline{0.8156}} & \textbf{\underline{0.6017}} & 1.0000 & 1.0000 & 1.0000 \\
&   & Decoder-only & 0.8944 & 0.7663 & 0.4888 & \underline{0.9442} & \underline{0.9415} & \underline{0.9370} \\
&   & VPT-shallow & 0.8112 & 0.7218 & 0.4889 & 0.8599 & 0.8605 & 0.8625 \\
&   & VPT-deep & 0.7995 & 0.7047 & 0.4695 & 0.8459 & 0.8466 & 0.8458 \\
&   & LoRA & 0.7775 & 0.6882 & 0.4870 & 0.7888 & 0.7952 & 0.8018 \\
&   & LoRA CKA aware & 0.8127 & 0.6593 & 0.3791 & 0.8314 & 0.8352 & 0.8390 \\
&   & LoRA Encoder-only & \textbf{\underline{0.9078}} & 0.7732 & 0.5253 & 0.8915 & 0.8887 & 0.8821 \\
&   & Full FT & 0.8991 & 0.7901 & 0.5014 & \textbf{0.9591} & \textbf{0.9568} & \textbf{0.9528} \\

\bottomrule
\end{longtable}
}
