# Supplementary material for: When Adaptation Hurts: Connecting Representational Drift to OOD Failures in MedSAM Fine-Tuning
Source: arXiv:2608.21300 source file (2026-08-29)
Supplement: Supplementary file 10 [file H_conclusion.tex]

\section{Appendix conclusions}
\label{subsec:appendix_conclusions}

Taken together, the additional analyses in the appendixes directly support the three contributions stated in the main paper. The bounding-box area statistics show that the same pixel-level jitter corresponds to very different effective prompt difficulty across datasets, especially for BUSI and CBIS-DDSM, which supports claim that robust evaluation must consider joint prompt noise and domain shift rather than idealized tight boxes alone. One method we proposed was jittered bounding box training, which generally improved robustness in- and ou-of-domain across adapted models. The degradation curves, heatmaps, and Dice gain tables further show that full fine-tuning and encoder-only LoRA provide the most favorable balance between in-domain adaptation and far-OOD robustness, while standard LoRA and VPT often improve target domain performance at the cost of much weaker generalization, especially under noisy prompts. Finally, the CKA analysis ties these outcomes to internal representation changes by showing that encoder similarity alone does not explain robustness, whereas preserving decoder and output representations is much more strongly associated with far-OOD performance. 
